# Supplementary material for: Local existence of smooth solutions for the semigeostrophic equations on curved domains
Source: arXiv:2206.06191 source file (2022-06-13)
Supplement: Supplementary file 1 [file appendices.tex]

\section{Sobolev embeddings and interpolation}\label{appendix:Sobolev_interpolation}
\begin{theorem}[Adams interpolation]\label{thm:Adams}Let $\Om\subset\R^n$ be any bounded and smooth domain. Then, for every $0\leq k\leq m$ there exists a constant $c=c(k,m,\Om)>0$ such that
\[
\norm{v}_{H^k(\Om)}\leq c\norm{v}_{L^2(\Om)}^{1-\frac{k}{m}}\norm{v}_{H^m(\Om)}^{\frac{k}{m}},
\]
for every $v\in H^m(\Om)$.
\end{theorem}
\begin{proof}
The detailed proof can be found in \cite[Chapter 5]{A08}. As a side remark, notice that the authors proved this result only assuming $\Om$ satisfying some suitable "weak cone condition".
\end{proof}
The following proposition is a small variation of Lemma 3.4  in \cite{MB01} (for our purposes, we specialize it from $\R^2$ to $\Om$. The proof is essentially the same).
\begin{proposition}[Interpolation inequalities]Let $\Om\subset \R^2$ be any smooth and bounded domain, and  let $v,w$ be functions in $H^r(\Om)$. Then, there exists $C=C(r,\Om)>0$ such that
\begin{equation}\label{eq:banach_algebra}
\norm{D^\alpha(vw)}_{L^2(\Om)}\leq C\Bigl(\norm{v}_{L^\infty(\Om)}\norm{w}_{H^r(\Om)}+\norm{w}_{L^\infty(\Om)}\norm{v}_{H^r(\Om)}\Bigr),
\end{equation}
for all multi-index $\abs{\alpha}=r$.
In particular, the following inequalities
\begin{equation}\label{eq:interpol_1}
\norm{D^\alpha (vw)-vD^\alpha w}_{L^2(\Om)}\leq C_r\Bigl(\norm{\nabla v}_{L^\infty(\Om)}\norm{w}_{H^{r-1}(\Om)}+\norm{v}_{H^r(\Om)}\norm{w}_{L^\infty(\Om)}\Bigr),
\end{equation}
and
\begin{equation}\label{eq:interpol_2}
\norm{D^\alpha(vw)-vD^\alpha w-wD^\alpha v}_{L^2(\Om)}\leq C_r\Bigl(\norm{\nabla v}_{L^\infty(\Om)}\norm{w}_{H^{r-1}(\Om)}+\norm{v}_{H^{r-1}(\Om)}\norm{\nabla w}_{L^\infty(\Om)}\Bigr),
\end{equation}
hold.
\end{proposition}
\begin{proof}
First of all, recall the following particular case of the Gagliardo-Nirenberg inequality: for every $r\geq 0$ there exists $C_r>0$ such that for every $i\leq r$ the following estimate
\begin{equation}\label{eq:GN}
\norm{D^i h}_{L^{2r/i}(\Om)}\leq C_r\norm{h}^{1-i/r}_{L^\infty(\Om)}\norm{D^r h}_{L^2(\Om)}^{i/r}+C_{r,\Om}\norm{h}_{L^2(\Om)},
\end{equation}
hold. Here, the last term compensate the fact that we consider a bounded and smooth domain $\Om$ instead of the whole plane $\R^2$  (see \cite[Page 126]{N60}).
Now, let $\abs{\alpha}=r$. By the Leibnitz rule and Hölder inequality we have that there exists $C_\alpha>0$ such that
\begin{align*}
\norm{D^\alpha(vw)}_{L^2(\Om)}\leq C_\alpha\sum_{\gamma+\beta=\alpha}\norm{D^\gamma vD^\beta w}_{L^2(\Om)}\leq C_\alpha\sum_{\gamma+\beta=\alpha}\norm{D^\gamma v}_{L^{\frac{2r}{\abs{\gamma}}}(\Om)}\norm{D^\beta w}_{L^{\frac{2r}{\abs{\beta}}}(\Om)},
\end{align*}
which, by \eqref{eq:GN}, we can estimate as
\begin{align*}
\norm{D^\alpha(vw)}_{L^2(\Om)}&\leq C_{\alpha,\Om}\sum_{\gamma+\beta=\alpha}\Bigl(\norm{v}_{L^\infty(\Om)}^{1-\frac{\abs{\gamma}}{r}}\norm{D^r v}_{L^2(\Om)}^{\frac{\abs{\gamma}}{r}}+\norm{v}_{L^2(\Om)}\Bigr)\Bigl(\norm{w}_{L^\infty(\Om)}^{1-\frac{\abs{\beta}}{r}}\norm{D^ r w}_{L^2(\Om)}^{\frac{\abs{\beta}}{r}}+\norm{w}_{L^2(\Om)}\Bigr)\\
&\leq C'_{\alpha,\Om}\sum_{i=0}^r\Biggl(\Bigl(\norm{v}_{L^\infty(\Om)}\norm{D^r w}_{L^2(\Om)}\Bigr)^{1-\frac{i}{r}}\Bigl(\norm{w}_{L^\infty(\Om)}\norm{D^r v}_{L^2(\Om)}\Bigr)^{\frac{i}{r}}\\
&\quad+\norm{w}_{L^2(\Om)}\norm{v}_{L^\infty(\Om)}^{1-\frac{i}{r}}\norm{D^r v}_{L^2(\Om)}^{\frac{i}{r}}+\norm{v}_{L^2(\Om)}\norm{w}_{L^\infty(\Om)}^{1-\frac{i}{r}}\norm{D^r w}_{L^2(\Om)}^{\frac{i}{r}}\Biggr)\\
&\leq C'_{\alpha,\Om}\Biggl(\Bigl(\norm{v}_{L^\infty(\Om)}\norm{D^r w}_{L^2(\Om)}+\norm{w}_{L^\infty(\Om)}\norm{D^r v}_{L^2(\Om)}\Bigr)\\
&\quad+\norm{w}_{L^2(\Om)}\Bigl(\norm{v}_{L^\infty(\Om)}+\norm{D^r v}_{L^2(\Om)}\Bigr)+\norm{v}_{L^2(\Om)}\Bigl(\norm{w}_{L^\infty(\Om)}+\norm{D^r w}_{L^2(\Om)}\Bigr)\Biggr).
\end{align*}
Since $\Om$ is bounded, then $L^\infty(\Om)\subset L^2(\Om)$, and therefore
\[
\norm{D^\alpha(vw)}_{L^2(\Om)}\leq C''_{\alpha,\Om}\Bigl(\norm{v}_{L^\infty(\Om)}\norm{w}_{H^r(\Om)}+\norm{w}_{L^\infty(\Om)}\norm{v}_{H^r(\Om)}\Bigr),
\]
for some $C''_{\alpha,\Om}>0$, proving \eqref{eq:banach_algebra}. Estimates \eqref{eq:interpol_1} and \eqref{eq:interpol_2} can be obtained in the exact same fashion simply observing that
\[
\norm{D^{\alpha}(vw)-vD^\alpha w}_{L^2(\Om)}\leq C_\alpha\sum_{\abs{\gamma}+\abs{\beta}\leq r-1}\norm{D^\gamma(\nabla v)D^\beta w}_{L^2(\Om)},
\] 
and
\[
\norm{D^{\alpha}(vw)-vD^\alpha w-wD^\alpha v}_{L^2(\Om)}\leq C_\alpha\sum_{\abs{\gamma}+\abs{\beta}\leq r-2}\norm{D^\gamma(\nabla v)D^\beta (\nabla w)}_{L^2(\Om)}.
\] 
\end{proof}
\begin{remark}In particular, if $r\geq 2$, Equation \eqref{eq:banach_algebra} implies that $H^r(\Om)$ is a Banach algebra, and if $\abs{\alpha}=r\geq 4$, then by the Sobolev embeddings $H^{2+s}(\Om)\hookrightarrow W^{s,\infty}(\Om)$ we have that
\begin{equation*}
\norm{D^\alpha (vw)-vD^\alpha w}_{L^2(\Om)}\leq C_r\norm{v}_{H^r(\Om)}\norm{w}_{H^{r-1}(\Om)},
\end{equation*}
and
\begin{equation*}
\norm{D^\alpha(vw)-vD^\alpha w-wD^\alpha v}_{L^2(\Om)}\leq C_r\norm{v}_{H^{r-1}(\Om)}\norm{w}_{H^{r-1}(\Om)}.
\end{equation*}
\end{remark}
